# Supplementary material for: Are We Ready for Real-Time LiDAR Semantic Segmentation in Autonomous Driving?
Source: arXiv:2410.08365 source file (2024-10-10)
Supplement: Supplementary file 1 [file X_suppl.tex]

\clearpage
\setcounter{page}{1}
\maketitlesupplementary

\section{Overview}
This supplementary material is organized as follows. We first provide the training protocol we employ in OpenNeuralPC in \cref{sec:trainingprotocol}, then provide a description for each dataset we target in \cref{sec:datasetsdescription}. Additionally, we provide per-class Intersection-over-Union (IoU) results of each evaluated model across the considered datasets in \cref{sec:semanticsegmentationresults}. Finally, we discuss the main differences between various NVIDIA Jetson platforms tuning configurations to different power modes in \cref{sec:additionalresults}, and then provide additional results on the AGX Orin and AGX Xavier considering their lowest power budget instead of the MAXN mode. 

\section{Training protocol}
\label{sec:trainingprotocol}
All models are reproduced and retrained through the OpenNeuralPC framework on a single NVIDIA GeForce RTX 4090 GPU with 24 GB of memory using AdamW optimizer for 45 epochs on SemanticKITTI~\cite{behley2019semantickitti} and nuScenes~\cite{caesar2020nuscenes} and for 100 epochs on ScanNetv2~\cite{dai2017scannet} (further training epochs have little to no impact), with a weight decay of 0.003, and a batch size of 3 (due to GPU memory capacity). For the learning rate, we use a scheduler with a linear warmup phase from 0 to 0.001 along the first 4 epochs and then a cosine annealing phase is used to decrease it to $10^{-5}$ at the end of the last epoch. The objective loss function used is a sum of the cross-entropy and the Lov\'{a}sz loss~\cite{berman2018lovaszsoftmaxloss}. To prevent overfitting, we implement classical point cloud augmentations: random rotation around the z-axis, random flip of the direction of the x-axis and y-axis, and random re-scaling (random translation is used instead of random re-scaling for SalsaNext~\cite{cortinhal2020salsanext} because re-scaling prior to projecting the point cloud to a LiDAR range image resulted in a poor performance).

Following~\cite{puy2023waffleiron, Xu2021rpvnet, Yan20222dpass}, we implement instance cutmix on SemanticKITTI~\cite{behley2019semantickitti}, specifically targeting rare-class objects in order to enhance segmentation performance on this dataset. The approach involves extracting instances from the following classes: bicycle, motorcycle, person, bicyclist, and other vehicles. During training, we randomly select up to 40 instances from each of the selected classes and apply various random transformations, including rotation around the z-axis, flipping along the x or y axes, and random re-scaling for each instance. These instances are then placed at random locations on roads, in parking areas, or on sidewalks.

\section{Datasets description}
\label{sec:datasetsdescription}
\textbf{SemanticKITTI~\cite{behley2019semantickitti}.}  This dataset showcases urban outdoor environments (i.e., city traffic, residential blocks, highways) captured with a Velodyne HDL-64E LiDAR covering the full 360\degree\ Field-of-View (FoV). We follow the same division of its 22 sequences, and only work with sequences 00 to 10 designated for training except for the 8$^{\text{th}}$ used for validation. In total, SemanticKITTI offers for training 19,130 complete 3D scans and for validation 4,071 ones, and provides point-wise annotations for 28 classes of which 25 are used to evaluate methods on semantic scene understanding.

\textbf{nuScenes~\cite{caesar2020nuscenes}.} It was the pioneering outdoor dataset that encompasses a comprehensive autonomous vehicle sensor suite including a Velodyne HDL-32E LiDAR, offering a complete 360\degree\ FoV while driving in Boston and Singapore, two cities very well known for their dense traffic and challenging driving situations. nuScenes offers 1000 scenes of 20s duration each, and provides 28,130 training scans and 6,019 validation ones all annotated with 32 classes, 16 of them used for evaluation.
 
\textbf{ScanNetv2~\cite{dai2017scannet}.}  This dataset provides 1,513 scans of more than 707 distinct indoor environments that are divided into 1,201 and 312 splits for training and validation, respectively. The acquisition sensor used is a Structure sensor, an RGB-D sensor with a design similar to the Microsoft Kinect v1. Additionally, voxel-wise annotations are provided for 20 classes all used for evaluation.

\section{Semantic segmentation results}
\label{sec:semanticsegmentationresults}
In this section, we provide per-class IoU results of the different models on SemanticKITTI, nuScenes, and ScanNetv2 in \cref{tab:semantickitti_iou}, \cref{tab:nuScenes_iou}, \cref{tab:scannetv2_iou}, respectively.
Our training protocol through OpenNeuralPC led to an increased segmentation accuracy for MinkUNet42~\cite{choy2019minkowski} and SPVCNN~\cite{tang2020spvnas} on SemanticKITTI. For instance, this increase is observed for MinkUNet42 particularly on the following classes: person (from 60.9 to 77.6), bicycle (from 40.4 to 59.8), bicyclist (from 61.9 to 89.3), and motorcycle (from 47.4 to 72.6) as previously reported in~\cite{tang2020spvnas}. This amelioration is largely attributed to the instance cutmix implemented on this dataset during the training phase.

\begin{table*}
\centering
\resizebox{\textwidth}{!}{
\setlength{\tabcolsep}{3pt}
 \begin{tabular}{>{\scriptsize}r >{\scriptsize}c >{\scriptsize}c >{\scriptsize}c >{\scriptsize}c >{\scriptsize}c >{\scriptsize}c >{\scriptsize}c >{\scriptsize}c >{\scriptsize}c >{\scriptsize}c >{\scriptsize}c >{\scriptsize}c >{\scriptsize}c >{\scriptsize}c >{\scriptsize}c >{\scriptsize}c >{\scriptsize}c >{\scriptsize}c >{\scriptsize}c >{\scriptsize}c >{\scriptsize}c >{\scriptsize}c }
\hline
 Method  
& \rotatebox{90}{ mIoU \%}
& \rotatebox{90}{ car} 
& \rotatebox{90}{ bicycle} 
& \rotatebox{90}{ motorcycle} 
& \rotatebox{90}{ truck} 
& \rotatebox{90}{ other-vehicle} 
& \rotatebox{90}{ person} 
& \rotatebox{90}{ bicyclist} 
& \rotatebox{90}{ motorcyclist} 
& \rotatebox{90}{ road}
& \rotatebox{90}{ parking}
& \rotatebox{90}{ sidewalk}
& \rotatebox{90}{ other-ground}
& \rotatebox{90}{ building}
& \rotatebox{90}{ fence}
& \rotatebox{90}{ vegetation}
& \rotatebox{90}{ trunk}
& \rotatebox{90}{ terrain}
& \rotatebox{90}{ pole}
& \rotatebox{90}{ traffic-sign} \\

\hline
\\[-2.2ex]
 \textbf{MinkNet~\cite{choy2019minkowski}}
&  64.3 \vrule
&  \underline{95.9} 
&  \textbf{59.8}
&  72.6 
&  62.1 
&  48.9 
&  \textbf{77.6} 
&  \underline{89.3} 
&  1.1
&  93.2
&  44.7
&  \underline{80.7}
&  2.2
&  89.6 
&  59.6  
&  87.5
&  65.5 
&  73.4
&  \textbf{65.5}
&  \textbf{51.6} \\

 \textbf{MinkNet\_0.5$\times$~\cite{choy2019minkowski}}
& 63.2 \vrule
& 95.4 
& 57.1
& 68.3 
& 63.9 
& 46.3 
& 75.4 
& 87.3 
& 2.0 
& 93.0 
& 44.9 
& 80.0 
& 2.7 
& 88.0 
& 54.2 
& 87.7 
& 65.4
& 74.4 
& 64.7 
& 50.6 \\

\textbf{SN\_64$\times$2048~\cite{cortinhal2020salsanext}}
& 55.9 \vrule
& 92.0
& 31.5
& 35.6
& 64.7
& \underline{49.4}
& 47.7
& 64.4
& 0.0
& 92.8
& 46.0
& 78.7
& 1.4
& 84.9
& 55.7
& 82.5
& 62.5
& 64.7
& 57.9
& 49.4 \\

\textbf{SN\_64$\times$1024~\cite{cortinhal2020salsanext}}
& 54.4 \vrule
& 90.9
& 28.4
& 33.5
& 64.7
& 49.3
& 37.8
& 55.1
& 0.0
& \underline{93.6}
& \underline{47.4}
& 78.7
& 0.9
& 85.0
& 58.1
& 81.9
& 59.9
& 65.0
& 57.5
& 46.7 \\

 \textbf{SPVCNN~\cite{tang2020spvnas}}
&  \underline{65.3} \vrule
&  \textbf{96.5}
&  \underline{58.1}
&  \textbf{77.3}
&  65.5 
&  \textbf{61.8}
&  \underline{77.3}
&  88.0
&  0.4
&  93.0
&  42.5
&  79.9
&  \underline{4.2} 
&  \underline{90.1}
&  \underline{62.2} 
&  87.5
&  \textbf{67.4}
&  73.6
&  \underline{65.4}
&  \underline{50.7} \\

 \textbf{SPVCNN\_0.5$\times$~\cite{tang2020spvnas}} 
& 63.4 \vrule
& 95.5
& 57.0
& 72.7
& 63.3
& 46.2
& 76.8
& 89.1
& 1.4
& 93.3
& 43.2
& 80.0
& 2.7
& 88.2
& 54.3
& 87.5
& 64.3 
& 74.0
& 64.4 
& 49.9 \\

\textbf{WI-48-256~\cite{puy2023waffleiron}}
&  \textbf{65.8} \vrule
&  95.4 
&  56.3 
&  \underline{75.3}
&  \textbf{83.8} 
&  41.9 
&  75.4 
&  \textbf{92.6} 
&  \textbf{4.8}
&  \textbf{94.6} 
&  \textbf{49.6} 
&  \textbf{82.1} 
&  1.5 
&  \textbf{91.1} 
&  \textbf{63.3} 
&  \underline{88.2} 
&  66.1 
&  \underline{75.7} 
&  63.7
&  48.7 \\

 \textbf{WI-12-128~\cite{puy2023waffleiron}}
&  63.6 \vrule
&  95.5 
&  50.9
&  68.0 
&  \underline{67.0} 
&  47.5 
&  70.0 
&  88.2 
&  \underline{3.4} 
&  \underline{93.6} 
&  44.7 
&  80.5 
&  \textbf{4.5} 
&  90.0 
&  59.1 
&  \textbf{88.9}
&  \underline{66.7} 
&  \textbf{77.4} 
&  63.2 
&  49.4 \\

\\[-2.2ex]
\hline
\end{tabular}
}
\caption{Semantic segmentation performance following our training protocol on SemanticKITTI validation set. The best and second best scores are in bold and underlined, respectively.}
\label{tab:semantickitti_iou}
\end{table*}

\begin{table*}
\centering
\resizebox{0.9\textwidth}{!}{
\setlength{\tabcolsep}{3pt}
 \begin{tabular}{>{\scriptsize}r >{\scriptsize}c >{\scriptsize}c >{\scriptsize}c >{\scriptsize}c >{\scriptsize}c >{\scriptsize}c >{\scriptsize}c >{\scriptsize}c >{\scriptsize}c >{\scriptsize}c >{\scriptsize}c >{\scriptsize}c >{\scriptsize}c >{\scriptsize}c >{\scriptsize}c >{\scriptsize}c >{\scriptsize}c >{\scriptsize}c >{\scriptsize}c }
\hline
Method  
& \rotatebox{90}{mIoU \%}
& \rotatebox{90}{barrier} 
& \rotatebox{90}{bicycle} 
& \rotatebox{90}{bus} 
& \rotatebox{90}{car} 
& \rotatebox{90}{const. veh.} 
& \rotatebox{90}{motorcycle} 
& \rotatebox{90}{pedestrian} 
& \rotatebox{90}{traffic cone} 
& \rotatebox{90}{trailer}
& \rotatebox{90}{truck}
& \rotatebox{90}{driv. surf.}
& \rotatebox{90}{other flat}
& \rotatebox{90}{sidewalk}
& \rotatebox{90}{terrain}
& \rotatebox{90}{manmade}
& \rotatebox{90}{vegetation} \\

\hline
\\[-2.2ex]

\textbf{MinkNet~\cite{choy2019minkowski}}
& 73.5 \vrule
& 74.5
& 39.8
& 89.7
& \textbf{91.0} 
& 44.3 
& \underline{78.7}
& \textbf{77.3}
& 60.4
& 56.7 
& \underline{82.6}
& 95.5 
& 68.8 
& 71.3 
& \textbf{74.4} 
& 86.1 
& \textbf{84.9} \\

\textbf{MinkNet\_0.5$\times$~\cite{choy2019minkowski}}
& 71.2 \vrule
& 72.5
& 28.9 
& 88.2
& \underline{90.0}
& 40.8
& 78.5
& 76.3
& 58.8
& 51.2
& 79.4
& 95.2 
& 66.2 
& 69.6 
& 73.4
& 85.4
& 84.3 \\

\textbf{SN\_32$\times$2048~\cite{cortinhal2020salsanext}}
& 68.2 \vrule
& 68.1 
& 15.2 
& 76.3 
& 85.4 
& 34.0 
& 73.5 
& 71.1 
& 57.1 
& 56.4 
& 72.4 
& 95.6 
& 70.0 
& 72.6 
& 72.9 
& 85.8 
& 84.3  \\

\textbf{SN\_32$\times$1024~\cite{cortinhal2020salsanext}}
& 69.2 \vrule
& 69.3
& 34.5 
& 77.5 
& 83.2 
& 28.7 
& 74.2 
& 67.8 
& 57.4 
& \underline{64.8} 
& 69.9 
& 95.5 
& 69.1 
& 72.8 
& 72.1 
& \textbf{86.4} 
& \underline{84.5}  \\

\textbf{SPVCNN~\cite{tang2020spvnas}}
& 72.6 \vrule
& 73.6
& \underline{40.8}
& 88.3 
& 88.6 
& 45.6
& 78.6
& 75.4 
& 59.4 
& 54.9 
& 82.3 
& 95.4 
& 67.3 
& 70.1
& 72.9 
& 85.4 
& 83.7 \\

\textbf{SPVCNN\_0.5$\times$~\cite{tang2020spvnas}}
& 69.6 \vrule
& 71.9 
& 34.8
& 85.0
& 88.1
& 39.1
& 72.5
& 73.4
& 55.6
& 48.1
& 80.0
& 94.9
& 62.9
& 68.1
& 71.7
& 84.5
& 83.0 \\

\textbf{WI-48-256~\cite{puy2023waffleiron}}
& \textbf{76.1} \vrule
& \textbf{77.8}
& \textbf{45.8} 
& \textbf{93.7}
& 85.3
& \textbf{50.2}
& \textbf{81.9}
& 75.8 
& \textbf{66.2} 
& \textbf{68.7}
& \textbf{83.2}
& \textbf{96.7} 
& \textbf{72.9} 
& \textbf{74.9}
& \underline{73.7} 
& \underline{86.3}
& 84.0 \\

\textbf{WI-12-128~\cite{puy2023waffleiron}}
& \underline{74.1} \vrule
& \underline{75.6}
& 40.1
& \underline{90.1}
& 88.1
& \underline{46.7}
& 77.7 
& \underline{76.6}
& \underline{61.9}
& 64.4
& 80.3 
& \underline{96.2}
& \underline{71.9} 
& \underline{73.4}
& 73.4
& 85.8
& 83.5 \\

\\[-2.2ex]
\hline
\end{tabular}
}
\caption{Semantic segmentation performance following our training protocol on nuScenes validation set. The best and second best scores are in bold and underlined, respectively.}
\label{tab:nuScenes_iou}
\end{table*}

\begin{table*}
\centering
\resizebox{\textwidth}{!}{
\setlength{\tabcolsep}{3pt}
 \begin{tabular}{>{\scriptsize}r >{\scriptsize}c >{\scriptsize}c >{\scriptsize}c >{\scriptsize}c >{\scriptsize}c >{\scriptsize}c >{\scriptsize}c >{\scriptsize}c >{\scriptsize}c >{\scriptsize}c >{\scriptsize}c >{\scriptsize}c >{\scriptsize}c >{\scriptsize}c >{\scriptsize}c >{\scriptsize}c >{\scriptsize}c >{\scriptsize}c >{\scriptsize}c >{\scriptsize}c >{\scriptsize}c }
\hline
 Method  
& \rotatebox{90}{ mIoU \%}
& \rotatebox{90}{ bathtub} 
& \rotatebox{90}{ bed} 
& \rotatebox{90}{ bookshelf} 
& \rotatebox{90}{ cabinet} 
& \rotatebox{90}{ chair} 
& \rotatebox{90}{ counter} 
& \rotatebox{90}{ curtain} 
& \rotatebox{90}{ desk} 
& \rotatebox{90}{ door}
& \rotatebox{90}{ floor}
& \rotatebox{90}{ otherfurniture}
& \rotatebox{90}{ picture}
& \rotatebox{90}{ refrigerator}
& \rotatebox{90}{ showercurtain}
& \rotatebox{90}{ sink}
& \rotatebox{90}{ sofa}
& \rotatebox{90}{ table}
& \rotatebox{90}{ toilet}
& \rotatebox{90}{ wall}
& \rotatebox{90}{ window} \\

\hline
\\[-2.2ex]

 \textbf{MinkNet~\cite{choy2019minkowski}}
& \underline{62.8} \vrule
& \underline{76.2}
& \textbf{93.8}
& 55.5
& \underline{74.9}
& \underline{87.2}
& 78.1
& \underline{66.4}
& \underline{39.8}
& \underline{49.5}
& \textbf{72.9}
& \underline{13.8}
& 56.1
& \underline{57.9} 
& 53.8
& \textbf{49.7}
& \textbf{62.1}
& \textbf{87.7}
& \underline{63.3}
& 76.8
& 40.7 \\

 \textbf{MinkNet\_0.5$\times$~\cite{choy2019minkowski}}
& 59.2 \vrule
& 74.2
& 93.6
& 51.5
& 68.7
& 85.4
& \textbf{80.3}
& 63.9
& 37.3
& 47.9
& 66.1
& 9.3
& 54.5 
& 52.5
& 48.9
& 41.8
& 51.1
& 83.3 
& 61.4
& 76.5
& 34.9 \\

 \textbf{SPVCNN~\cite{tang2020spvnas}}
& \textbf{64.1} \vrule
& \textbf{77.4}
& \underline{93.7}
& \textbf{58.8}
& \textbf{75.4}
& \textbf{87.3} 
& \underline{79.5}
& \textbf{67.2}
& \textbf{41.8}
& \textbf{53.0}
& \underline{71.8}
& \textbf{15.7}
& \underline{60.1}
& \textbf{60.3}
& \textbf{57.6} 
& 43.7
& \underline{58.9}
& \underline{86.9}
& \textbf{65.9}
& \underline{79.3}
& \textbf{47.6} \\

 \textbf{SPVCNN\_0.5$\times$~\cite{tang2020spvnas}}
& 61.6 \vrule
& \underline{76.2}
& 93.5 
& \underline{55.9}
& 72.9
& 85.7
& 77.4
& 65.1
& 39.1
& \underline{49.5}
& 68.5
& 10.6
& \textbf{61.4}
& 54.7
& \underline{56.9}
& \underline{46.0}
& 52.0
& 80.5
& 60.2
& \textbf{80.2}
& \underline{45.5} \\

 \textbf{WI-48-256~\cite{puy2023waffleiron}}
& 46.4 \vrule
& 66.6
& 91.4
& 44.2
& 60.5
& 69.4
& 58.1
& 57.2
& 18.9
& 38.5
& 48.1
& 4.7
& 46.8
& 43.2
& 36.4
& 25.0
& 34.1
& 58.0
& 44.4
& 61.0
& 21.7 \\

 \textbf{WI-12-128~\cite{puy2023waffleiron}}
& 43.0 \vrule
& 66.5
& 91.2
& 39.3
& 57.8
& 66.7 
& 53.7
& 54.6
& 19.2
& 35.4 
& 44.1
& 3.6
& 45.0
& 38.8
& 37.2
& 22.8
& 28.4
& 47.4
& 42.6 
& 50.9
& 15.1 \\

\\[-2.2ex]
\hline
\end{tabular}
}
\caption{Semantic segmentation performance following our training protocol on ScanNetv2 validation set. The best and second best scores are in bold and underlined, respectively.}
\label{tab:scannetv2_iou}
\end{table*}

\section{Additional results on NVIDIA Jetson}
\label{sec:additionalresults}
Power consumption and battery usage are two important aspects to assess the efficiency of a neural network on a robotic system. Inferring complex and deep neural networks on resource-constrained devices can draw a substantial amount of the system's provided power. However, in scenarios where a limiting power budget is imposed, the performance of such models becomes a critical concern, particularly when deployed on embedded systems. Therefore, in this section, we investigate the impact of the power limitation on the computational capabilities of the Jetson platforms and overall operational efficiency of the considered neural networks; thus, providing insights on the integration of such models within the given power constraints of NVIDIA embedded systems. We present in \cref{tab:jetson_tuning} the different NVIDIA Jetson tuning configurations that we adopt in our experiments. The main system components that differ between the MAXN power configuration and the lowest power budget of each considered Jetson platform are the number of active CPU cores, and corresponding CPU/GPU maximum frequencies. Further, we provide additional performance results on the lowest power budget of each platform in \cref{tab:performance_metrics_lowpower}. Overall, the findings reveal a much lower power draw of all models in terms of CPU and GPU, but at the cost of a significant increase in both Pre-Processing and Inference time from the MAXN configuration, and hence the Total Runtime for all models across all datasets, which further hinders their real-time execution. As for the peak allocated GPU memory, it remains unaffected. 
\begin{table}[H]
\centering
\resizebox{0.47\textwidth}{!}{
\begin{tabular}{|c|c|c|c|c|}
\cline{2-5}
\multicolumn{1}{c|}{} & \multicolumn{2}{c|}{\textbf{AGX Orin}} & \multicolumn{2}{c|}{\textbf{AGX Xavier}} \\
\hline
\textbf{Power Mode} & \textbf{MAXN} & \textbf{15W} & \textbf{MAXN} & \textbf{10W} \\
\hline
\textbf{Online CPU cores} & 12 & 4 & 8 & 2 \\
\hline
\textbf{CPU Max} & \multirow{2}{*}{2,201.6} & \multirow{2}{*}{1,113.6} & \multirow{2}{*}{2,265.6} & \multirow{2}{*}{1,200} \\
\textbf{Frequency (MHz)} & & & &  \\
\hline

\textbf{GPU Max} & \multirow{2}{*}{1,301} & \multirow{2}{*}{408} & \multirow{2}{*}{1,377} & \multirow{2}{*}{520} \\
\textbf{Frequency (MHz)} & & & &  \\
\hline
\end{tabular}
}
\caption{Performance tuning of the considered NVIDIA Jetson platforms. MAXN represents the limits and therefore has no power budget.}
\label{tab:jetson_tuning}
\end{table}

\begin{table*}[t] % [t] to pin the table at the top
  \centering
  \resizebox{\textwidth}{!}{
  
  \begin{tabular}{|c|c|c|r@{ }r@{}c@{ }c@{}r@{}l|r@{ }c@{}r@{ }c@{}r@{}l|c|c|r@{ }r@{}c@{ }c@{}r@{}l|r@{ }c@{}r@{ }c@{}r@{}l|}
    \cline{3-29}
    \multicolumn{2}{c|}{} &  & \multicolumn{12}{c|}{\textbf{Total Runtime}} & \multicolumn{2}{c|}{\textbf{GPU Memory}} & \multicolumn{12}{c|}{\textbf{Total Power}}\\

    \multicolumn{2}{c|}{} & \textbf{mIoU} & \multicolumn{12}{c|}{(Pre-Processing + Inference) \textbf{(ms)}} & \multicolumn{2}{c|}{\textbf{(MB)}} & \multicolumn{12}{c|}{(CPU + GPU) \textbf{(W)}}\\
    
    \cline{4-29}
    \multicolumn{2}{c|}{} & \textbf{\%} & \multicolumn{6}{c|}{\textbf{Orin 15W}}  & \multicolumn{6}{c|}{\textbf{Xavier 10W}} & \textbf{Orin}  & \textbf{Xavier} & \multicolumn{6}{c|}{\textbf{Orin 15W}}  & \multicolumn{6}{c|}{\textbf{Xavier 10W}}\\
    
    \hline
    \multirow{8}{*}{\rotatebox[origin=c]{90}{\begin{tabular}{@{}c@{}}\textbf{SemanticKITTI} \\ \textbf{Validation~\cite{behley2019semantickitti}}\end{tabular}}} & \textbf{MinkNet~\cite{choy2019minkowski}} & 64.3 & \textbf{853} & ( & 79 & + & 774 & ) & \textbf{1,134} & ( & 125 & + & 1,009 & ) & 542 & 542 & \textbf{5.7} & ( & 0.8 & + & 4.9 & ) & \textbf{4.4} & ( & 0.8 & + & 3.6 & )\\
    \cline{2-29}
    & \textbf{MinkNet\_0.5$\times$~\cite{choy2019minkowski}} & 63.2 & \textbf{536} & ( & 79 & + & 457 & ) & \textbf{705} & ( & 120 & + & 585 & ) & 266 & 266 & \textbf{5.3} & ( & 0.8 & + & 4.5 & ) & \textbf{4.1} & ( & 0.8 & + & 3.3 & )\\
    
    \cline{2-29}
    & \textbf{SN\_64$\times$2048~\cite{cortinhal2020salsanext}} & 55.9 & \textbf{411} & ( & 143 & + & 268 & ) & \textbf{812} & ( & 217 & + & 595 & ) & 471 & 365 & \textbf{6.0} & ( & 0.8 & + & 5.2 & ) & \textbf{4.4} & ( & 0.8 & + & 3.6 & )\\
    \cline{2-29}
    & \textbf{SN\_64$\times$1024~\cite{cortinhal2020salsanext}} & 54.4 & \textbf{265} & ( & 126 & + & 139 & ) & \textbf{497} & ( & 194 & + & 303 & ) & 320 & 198 & \textbf{5.5} & ( & 0.8 & + & 4.7 & ) & \textbf{4.1} & ( & 0.9 & + & 3.2 & )\\

    \cline{2-29}
    & \textbf{SPVCNN~\cite{tang2020spvnas}} & 65.3 & \textbf{1,025} & ( & 80 & + & 945 & ) & \textbf{1,338} & ( & 117 & + & 1,221 & ) & 657 & 657 & \textbf{5.6} & ( & 0.8 & + & 4.8 & ) & \textbf{4.1} & ( & 0.7 & + & 3.4 & )\\
    \cline{2-29}
    & \textbf{SPVCNN\_0.5$\times$~\cite{tang2020spvnas}} & 63.4 & \textbf{672} & ( & 79 & + & 593 & ) & \textbf{857} & ( & 114 & + & 743 & ) & 343 & 343 & \textbf{5.4} & ( & 0.8 & + & 4.6 & ) & \textbf{3.6} & ( & 0.8 & + & 2.8 & )\\

    \cline{2-29}
     & \textbf{WI-48-256~\cite{puy2023waffleiron}} & 65.8 & \textbf{8,664} & ( & 728 & + & 7,936 & ) & \textbf{9,763} & ( & 993 & + & 8,770 & ) & 2,384 & 2,378 & \textbf{5.6} & ( & 0.8 & + & 4.8 & ) & \textbf{4.2} & ( & 0.7 & + & 3.5 & )\\
    \cline{2-29}
    & \textbf{WI-12-128~\cite{puy2023waffleiron}} & 63.6 & \textbf{1,779} & ( & 705 & + & 1,074 & ) & \textbf{2,282} & ( & 976 & + & 1,306 & ) & 1,186 & 1,178 & \textbf{5.0} & ( & 0.8 & + & 4.2 & ) & \textbf{3.6} & ( & 0.8 & + & 2.8 & )\\
    
    \hline
    \hline
    
    \multirow{8}{*}{\rotatebox[origin=c]{90}{\begin{tabular}{@{}c@{}}\textbf{nuScenes} \\ \textbf{Validation~\cite{caesar2020nuscenes}}\end{tabular}}}   & \textbf{MinkNet~\cite{choy2019minkowski}} & 73.5 & \textbf{286} & ( & 37 & + & 249 & ) & \textbf{365} & ( & 63 & + & 302 & ) & 351 & 351 & \textbf{5.3} & ( & 1.1 & + & 4.2 & ) & \textbf{3.9} & ( & 0.9 & + & 3.0 & )\\
    \cline{2-29}
    & \textbf{MinkNet\_0.5$\times$~\cite{choy2019minkowski}} & 71.2 & \textbf{255} & ( & 37 & + & 218 & ) & \textbf{263} & ( & 60 & + & 203 & ) & 128 & 128 & \textbf{5.0} & ( & 1.2 & + & 3.8 & ) & \textbf{3.5} & ( & 1.0 & + & 2.5 & )\\
    
    \cline{2-29}
    & \textbf{SN\_32$\times$2048~\cite{cortinhal2020salsanext}} & 68.2 & \textbf{229} & ( & 88 & + & 141 & ) & \textbf{429} & ( & 121 & + & 308 & ) & 317 & 196 & \textbf{5.9} & ( & 0.8 & + & 5.1 & ) & \textbf{4.3} & ( & 0.9 & + & 3.4 & )\\
    \cline{2-29}
    & \textbf{SN\_32$\times$1024~\cite{cortinhal2020salsanext}} & 69.2 & \textbf{156} & ( & 82 & + & 74 & ) & \textbf{283} & ( & 116 & + & 167 & ) & 240 & 113 & \textbf{5.7} & ( & 1.0 & + & 4.7 & ) & \textbf{4.1} & ( & 0.9 & + & 3.2 & )\\
    
    \cline{2-29}
    & \textbf{SPVCNN~\cite{tang2020spvnas}} & 72.6 & \textbf{382} & ( & 38 & + & 344 & ) & \textbf{464} & ( & 60 & + & 404 & ) & 383 & 383 & \textbf{5.1} & ( & 1.0 & + & 4.1 & ) & \textbf{3.8} & ( & 0.9 & + & 2.9 & )\\
    \cline{2-29}
    & \textbf{SPVCNN\_0.5$\times$~\cite{tang2020spvnas}} & 69.6 & \textbf{341} & ( & 38 & + & 303 & ) & \textbf{354} & ( & 59 & + & 295 & ) & 149 & 149 & \textbf{4.9} & ( & 1.1 & + & 3.8 & ) & \textbf{3.5} & ( & 0.9 & + & 2.6 & )\\

    \cline{2-29}
    & \textbf{WI-48-256~\cite{puy2023waffleiron}} & 76.1 & \textbf{2,271} & ( & 211 & + & 2,060 & ) & \textbf{2,586} & ( & 292 & + & 2,294 & ) & 750 & 747 & \textbf{5.4} & ( & 0.8 & + & 4.6 & ) & \textbf{4.1} & ( & 0.7 & + & 3.4 & )\\
    \cline{2-29}
    & \textbf{WI-12-128~\cite{puy2023waffleiron}} & 74.1 & \textbf{526} & ( & 197 & + & 329 & ) & \textbf{665} & ( & 298 & + & 367 & ) & 349 & 347 & \textbf{4.9} & ( & 0.8 & + & 4.1 & ) & \textbf{3.6} & ( & 0.9 & + & 2.7 & )\\
    
    \hline
    \hline
    
    \multirow{6}{*}{\rotatebox[origin=c]{90}{\begin{tabular}{@{}c@{}}\textbf{ScanNetv2} \\ \textbf{Validation~\cite{dai2017scannet}}\end{tabular}}} 
    & \textbf{MinkNet~\cite{choy2019minkowski}} & 62.8 & \textbf{433} & ( & 103 & + & 330 & ) & \textbf{525} & ( & 155 & + & 370 & ) & 458 & 450 & \textbf{4.9} & ( & 0.8 & + & 4.1 & ) & \textbf{3.8} & ( & 0.9 & + & 2.9 & )\\
    \cline{2-29}
    & \textbf{MinkNet\_0.5$\times$~\cite{choy2019minkowski}} & 59.2 & \textbf{354} & ( & 103 & + & 251 & ) & \textbf{395} & ( & 144 & + & 251 & ) & 214 & 206 & \textbf{4.6} & ( & 0.8 & + & 3.8 & ) & \textbf{3.5} & ( & 0.9 & + & 2.6 & )\\
    
    \cline{2-29}
    & \textbf{SPVCNN~\cite{tang2020spvnas}} & 64.1 & \textbf{496} & ( & 108 & + & 388 & ) & \textbf{584} & ( & 142 & + & 442 & ) & 546 & 535 & \textbf{4.9} & ( & 0.8 & + & 4.1 & ) & \textbf{3.8} & ( & 0.9 & + & 2.9 & )\\
    \cline{2-29}
    & \textbf{SPVCNN\_0.5$\times$~\cite{tang2020spvnas}} & 61.6 & \textbf{401} & ( & 104 & + & 297 & ) & \textbf{445} & ( & 137 & + & 308 & ) & 269 & 263 & \textbf{4.7} & ( & 0.8 & + & 3.9 & ) & \textbf{3.5} & ( & 0.9 & + & 2.6 & )\\

    \cline{2-29}
    & \textbf{WI-48-256~\cite{puy2023waffleiron}} & 46.4 & \textbf{1,789} & ( & 563 & + & 1,226 & ) & \textbf{2,084} & ( & 743 & + & 1,341 & ) & 745 & 737 & \textbf{5.0} & ( & 0.8 & + & 4.2 & ) & \textbf{3.7} & ( & 0.8 & + & 2.9 & )\\
    \cline{2-29}
    & \textbf{WI-12-128~\cite{puy2023waffleiron}} & 43.0 & \textbf{762} & ( & 562 & + & 200 & ) & \textbf{981} & ( & 742 & + & 239 & ) & 352 & 345 & \textbf{4.4} & ( & 0.9 & + & 3.5 & ) & \textbf{3.1} & ( & 0.9 & + & 2.2 & )\\
    
    \hline
  \end{tabular}
  }
  \caption{Performance metrics evaluated over 1000 scans from the validation set of SemanticKITTI and nuScenes and over 311 scans from the validation set of ScanNetv2, using a batch size of 1 and performed on different computing architectures. The mean values of Total Runtime, Pre-Processing, and Inference are presented with a standard deviation not exceeding 10\% for SemanticKITTI and nuScenes, and within 17\%--56\% for ScanNetv2 of the respective values. The Pre-Processing also encompasses the Post-Processing, but since the latter is less significant in comparison, we adopt the Pre-Processing naming convention. The peak allocated GPU memory is reported, and the RAM memory recordings do not exceed 45 MB on SemanticKITTI, 25 MB on nuScenes, and 70 MB on ScanNetv2 for all models. In the Total Power, the CPU readings also include PVA + DLA power consumption, and the GPU readings also include SOC power consumption.}
  \label{tab:performance_metrics_lowpower}
\end{table*}
